# Supplementary material for: Learning 3D Part Assembly from a Single Image
Source: arXiv:2003.09754 source file (2020-03-24)
Supplement: Supplementary file 1 [file fig-supp-arch-detail.tex]

\begin{figure}[!tbp]
    \centering
    \begin{minipage}{.4\linewidth}
    \input{fig/tab_arch_mask}
    \end{minipage}
    \hfill
    \begin{minipage}[b]{.4\linewidth}
    \input{fig/tab_arch_pose}
    \end{minipage}
\end{figure}
